# Supplementary material for: See through Gradients: Image Batch Recovery via GradInversion
Source: arXiv:2104.07586 source file (2021-04-15)
Supplement: Supplementary file 1 [file suppl_new.tex]

\section*{Supplementary Materials - A}
We provide more experimental details in the following sections.

\paragraph{$\mathcal{L}_{grad}$ cost function.} For the task of gradient matching, we study how the loss function affects optimization in Table~\ref{tb:loss_ablation_table}. 
We find $\ell_2$ loss outperforms cosine similarity~\cite{geiping2020inverting} for gradient matching. To this end, we compare the $\ell_2$ distance, percentage of gradient signs that matched, and the cosine similarity between the final optimized gradient and the ground truth gradient. It can be observed that an $\ell_2$ regularization results in stronger convergence for this task. 
\input{tables/cosine_table}

% \paragraph{Sensitivity to pre-processing.} Unlike our observations with DeepInversion, gradient matching is highly sensitive to pre-processing. A quick example is summarized in Table~\ref{}. We consequentially disabled all such steps.

% \input{tables/preprocessing}

\paragraph{Ablation studies qualitative results.}

We provide detailed visual comparison of the batch in ablation studies in Fig.~\ref{fig:ablation_imgs}.

\paragraph{Additional visual examples for privacy leakage.} We include more feature leakage examples in Fig.~\ref{fig:more_and_more}.

\paragraph{Insights \& Open challenges.} In our experiments, we observe the existence of several interesting facts of gradient inversion that may provide insights to future directions.
\begin{itemize}
    \item \textbf{Vanishing objects.} GradInverson can yield very similar images to original while come certain objects are missing as a whole. Interestingly this is in line as observation in latent code projection \etal~\cite{karras2020analyzing}.
    
    \item \textbf{Texts \& digits.} We observe gradient inversion reverses out existence of digits and letters, but not yet completely readable and remains private.
    
    \item \textbf{Human faces.} GradInversion still faces challenges with harder classes in ImageNet that involves human faces. Though reversing out segments of human faces, \eg mouths, eyes, and eyes, accurately relocating them in correct positions remain challenging. 
\end{itemize}

\input{figures/missing_objects}
% \noindent
% \textbf{With and without original BN statistics.}
% We next consider the case where without the original BN statistics and present the results in Table~\ref{tab:no_bn}. We observe an increased LPIPS at $0.642$, where we conjecture the BN statistic estimation may suffer differences when batch size is far beyond the original training batch size. However, DeepInversion$_{grad}$ still reveals image-level privacy, as shown in Fig.~\ref{fig:no_bn}. 

% \include{figures/no_bn}

\input{figures/main_results_image_ablation}

\input{figures/more_images}
